# Supplementary material for: On the Evaluation and Real-World Usage Scenarios of Deep Vessel Segmentation for Retinography
Source: arXiv:1909.03856 source file (2020-03-17)
Supplement: Supplementary file 1 [file covdappendix.tex]

\begingroup
\setlength\tabcolsep{4pt} % default value: 6pt
\begin{table}[htb]
\caption{Comparison of $F1_{micro}$-Scores (std) of DRIU and M2U-Net on COVD$-$ and COVD$-$SSL. Standard deviation across test-images in brackets.}
\label{tab:driuappendix}
\begin{center}
\begin{tabular}{@{}lllll@{}}
\toprule
Source   & Target     & DRIU            & DRIU BN         & M2U-Net         \\ \midrule
COVD$-$    & DRIVE      & 0.788 (0.018) & 0.797 (0.019) & \textbf{0.789} (0.018) \\
COVD$-$SSL & DRIVE      & 0.785 (0.018) & 0.783 (0.019) & \textbf{0.791} (0.014) \\
COVD$-$    & STARE      & 0.778 (0.117) & 0.778 (0.122) & \textbf{0.812} (0.046) \\
COVD$-$SSL & STARE      & 0.788 (0.102) & 0.811 (0.074) & \textbf{0.820} (0.044) \\
COVD$-$    & CHASE\_DB1 & \textbf{0.796} (0.027) & 0.791 (0.025) & 0.788 (0.024) \\
COVD$-$SSL & CHASE\_DB1 & 0.796 (0.024) & 0.798 (0.025) & \textbf{0.799} (0.026) \\
COVD$-$    & HRF        & 0.799 (0.044) & 0.800 (0.045) & \textbf{0.802} (0.045) \\
COVD$-$SSL & HRF        & \textbf{0.799} (0.044) & 0.784 (0.048) & 0.797 (0.044) \\
COVD$-$    & IOSTAR     & 0.791 (0.021) & 0.777 (0.032) & \textbf{0.793} (0.015) \\
COVD$-$SSL & IOSTAR     & \textbf{0.791} (0.021) & 0.811 (0.074) & 0.785 (0.018) \\ \bottomrule
\end{tabular}
\end{center}
\end{table}
\endgroup
